# Supplementary material for: Recognizing Developers' Emotions while Programming
Source: arXiv:2001.09177 source file (2021-05-06)
Supplement: Supplementary file 1 [file appendix.tex]

\section{Appendices}

%\begin{verbatim}
%  \appendix
%\end{verbatim}

%
% The acknowledgments section is defined using the "acks" environment (and NOT an unnumbered section). This ensures
% the proper identification of the section in the article metadata, and the consistent spelling of the heading.
